# Supplementary material for: Tunable Hybridization Between Electronic States of Graphene and Physisorbed Hexacene
Source: arXiv:1507.08381 source file (2015-07-30)
Supplement: Supplementary file 1 [file SI.pdf]

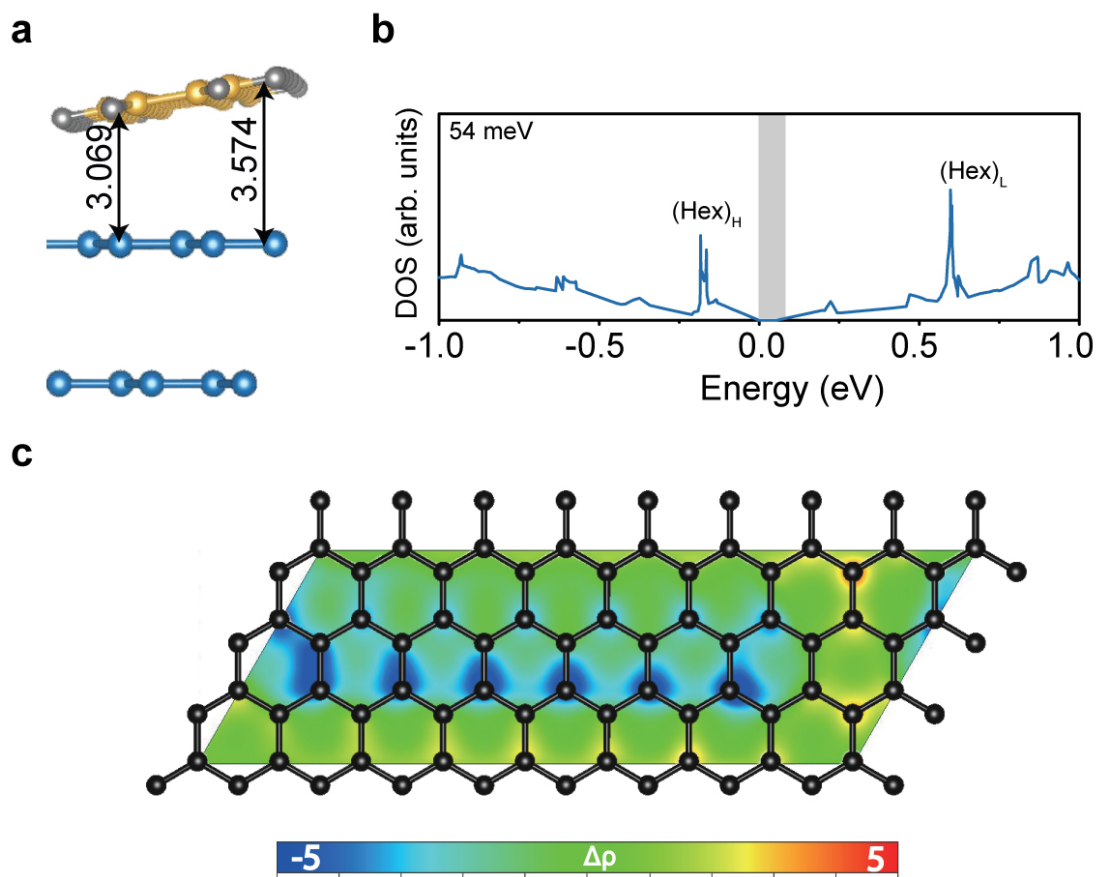

**Figure S1.** Single-molecular adsorption of hexacene on bilayer graphene at a high ( $1.31 \times 10^{-10} \text{ mol}/\text{cm}^2$ ) molecular concentration. (a) Adsorption geometry with  $11^\circ$  tilt angle. (b) PDOS of bilayer graphene. The grey region indicates a 54 meV band gap, the Fermi level is set to zero. (c) Charge density difference along a plane parallel to the basal plane of graphene. The position of the cutplane is  $0.62 \text{ \AA}$  above the top graphene layer. The color bar indicates the level of isosurface (unit in  $10^{-4} \text{ e}/\text{\AA}^3$ ).

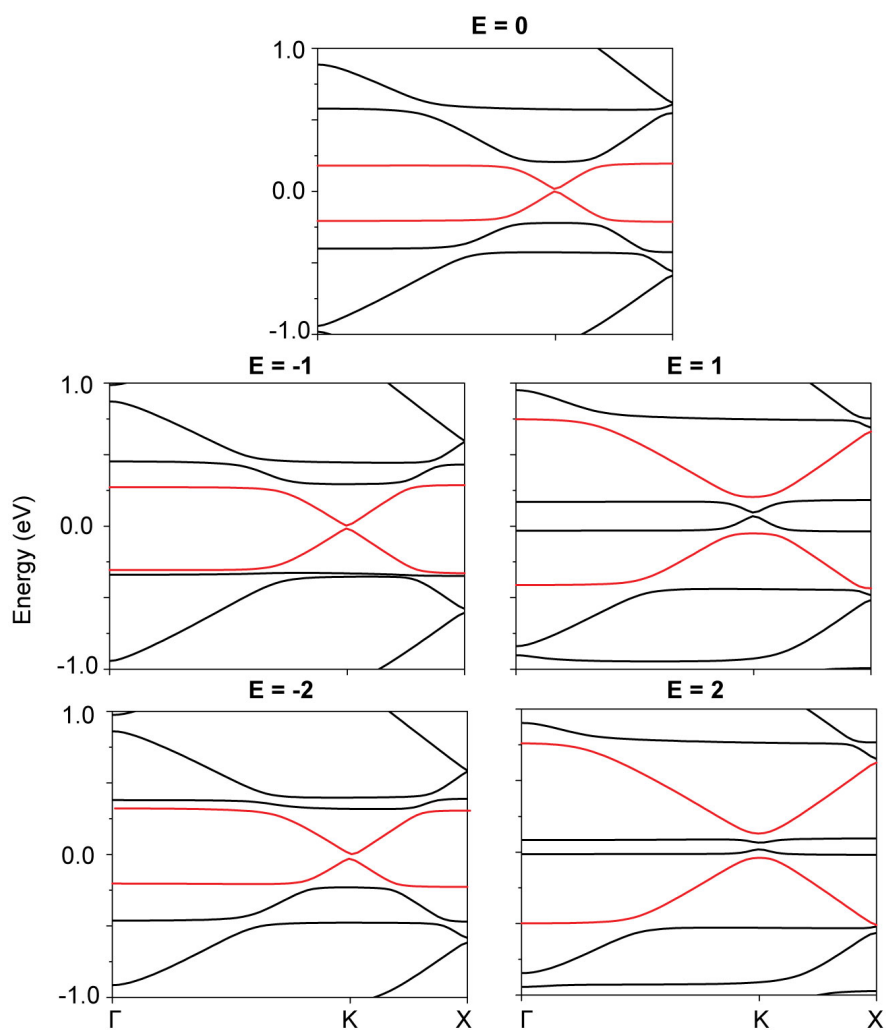

**Figure S2.** Electronic band structure diagrams for dual-molecular adsorption of hexacene and perfluorohexacene with monolayer coverage on monolayer graphene as a function of the strength of the electric field (in eV/nm). The  $\pi$  and  $\pi^*$  bands of bilayer graphene are labelled in red color.
